# Supplementary material for: Dynamic borrowing from historical controls via the synthetic prior with covariates in randomized clinical trials
Source: arXiv:2410.07242 ancillary file (2025-07-31)
Supplement: Supplementary file 1 [file supplement.pdf]

# Dynamic borrowing from historical controls via the synthetic prior with covariates in randomized clinical trials

## Supporting Information

Daniel E. Schwartz<sup>1</sup>, Yuan Ji<sup>1</sup>, and Li Wang<sup>2</sup>

<sup>1</sup>University of Chicago

<sup>2</sup>Abbvie

## 1 Data generation details for the simulation study

### 1.1 Factors defining the different simulation settings

In the simulation study data are generated according in a wide array of schemes, which consists of a (nearly) full factorial design with the following factors.

*Direct relevance of historical rates and usefulness of covariates.* The most important conditions we vary across simulations are (a) whether the historical control rates are directly relevant (similar) to the new rate or not and (b) whether the covariates predict response rates or not. These conditions define what we call Scenarios 1-4:

- Scenario 1: Historical rates similar to new rate *and* covariates predictive
- Scenario 2: Historical rates not similar but covariates predictive

- Scenario 3: Historical rates similar and covariates not predictive
- Scenario 4: Historical rates not similar and covariates not predictive

For further details see the beginning of Section 1.2 and the attached code/simulated historical data files.

*Maximum target control group size.* The maximum target control group size may be either 150 or 80 patients, reflecting some of the range of sample sizes typical in non-oncology Phase 2 efficacy trials (see, e.g., Table 5). In the designs we consider 150 or 80 are also the *fixed* sample sizes of the treatment group, with equal randomization between treatment and control in Stage 1 and unbalanced randomization in Stage 2 (depending on the # of Stage 2 control patients). This leads to total trial sizes on the order of 300 or 160, more or less depending on the concordance between the historical and new control data at interim.

*Whether all covariates are used.* The data-generating schemes for the main simulation results in Tables 1 and 3 are given by a full factorial design defined on the *previous* factors, in a setting where the analyst only observes and uses 2 of the 6 covariates actually associated with response rates. Finally, just for Scenarios 1 and 2 (where covariates are useful) and the  $n_{max}^c = 150$  maximum trial size case, we also simulate cases in which the analysts observe and may use all 6 covariates, yielding Tables and 4.

## 1.2 Exact sampling procedure

We directly generate trial-level data without sampling any patient-level data. To generate random trial-level covariates and true response rates that are correlated, we first sample from a marginal distribution for the covariates and then from a conditional distribution for response rates given covariates.

All the basic Scenarios 1-4 use the same historical data set, except that in Scenarios 3 and 4 the covariates are permuted across trials to break their correlation with the outcome. To sample the covariates for this data set of 15 trials, we sampled 3 trials each from 5 different groups, each having a different covariate distribution.

To sample a single trial's control data:

1. Sample covariates.

The trial-level covariates include both patient characteristics, which are randomly sampled, and trial eligibility or treatment regimen features, which are fixed under repeated sampling for a given trial (but vary deterministically across trials). To reflect a setting where different trials (indexed by  $h \in \{1, \dots, 15\}$ ) are conducted in different settings, we pose 5 different covariate distributions and each trial's covariates are sampled from just one of these 5 (indexed by the function  $i(h) \in \{1, \dots, 5\}$ ).

- Average disease duration at trial start (years):

$$\sim \mu_{i(h)} + \begin{cases} -2 & w.p. \ 0.15 \\ -1 & w.p. \ 0.2 \\ 0 & w.p. \ 0.3 \\ 1 & w.p. \ 0.2 \\ 2 & w.p. \ 0.15 \end{cases}$$

where  $\mu_{i(h)}$  is the  $i(h)$ -th component of the vector  $(20, 11, 16, 22, 16)$ .

- Previous/background treatment at trial start:

$$= b_{i(h)}$$

where  $b_{i(h)}$  is the  $i(h)$ -th component of the vector

(none, none, MTX, MTX, none).

2. Set trial control group size.

The control group sizes of the historical trials were determined jointly with the covariates, with

$$n_h = s_{i(h)}$$

where  $s_{i(h)}$  is the  $i(h)$ -th component of the vector  $(50, 200, 110, 40, 60)$ .

3. Sample observed response rate given covariates.

$$y_h|\psi_h \stackrel{ind.}{\sim} \text{Binom}(n_h, \psi_h)$$

$$\psi_h = \text{logit}^{-1} (0.2 \log 0.65 \cdot \text{duration}_h + \log 1.6 \cdot \text{MTX}_h)$$

where  $\text{duration}_h$  denotes the average disease duration at trial start of patients in trial  $h$ , and  $\text{MTX}_h$  is an indicator denoting whether or not trial  $h$  studied patients previously treated with MTX (1) or not (0).

These covariate distributions and regression equation were calibrated to mimic the range of covariate values and response rates we observed in an expanded version of Table 5.

To sample the new trial’s treatment group data we take

$$y_{trt}|\psi_{trt} \sim \text{Bin}(n_{trt}, \psi_{trt})$$

where  $n_{trt}$  is the control group’s maximum target sample size (half for interim analysis) and  $\psi_{trt}$  is 0 or 0.3 greater than the new trial’s control rate of  $\psi_{H+1}$  (reflecting no treatment effect or an additive treatment effect of 30 percentage points).

For the Frequentist repeated sampling in the simulation study, we sampled the historical trials’ data *just once* for each of Scenarios 1-4 and fixed it under repeated sampling. For the new trial’s data, we fixed the covariate values ( $\text{duration}_{H+1} = 16$  and  $\text{MTX}_{H+1} = 0$  in Scenarios 1 and 3 and  $\text{duration}_{H+1} = 8$  and  $\text{MTX}_{H+1} = 1$  in Scenarios 2 and 4) and only randomly the outcome, using the binomial regression above. This reflects a setting where the historical trials have already been run, and the Frequentist replication being considered is just replication of the yet-to-be conducted new trial. The fixed historical data set that was generated for each Scenario is shared along with the code.

## 2 Simulation results for variations on the SPx prior

In Table S1 we give simulation results from Table 1, with the addition of those for two minor variations on the original SPx prior.

“SPx C.” stands for “SPx Careful”, and mimics the SPx prior stated in Section 2.2

but with

$$(p_{hist}, p_{reg}, p_{ind}) = \left( \frac{3}{40}, \frac{3}{40}, \frac{34}{40} \right)$$

instead of  $(p_{hist}, p_{reg}, p_{ind}) = (\frac{1}{8}, \frac{1}{8}, \frac{3}{4})$ , giving the no-borrowing submodel 85% prior weight instead of 75%.

“SPx D.” stands for “SPx Diffuse”, and it puts equal prior weights on the submodels while making the priors within the borrowing submodels more diffuse (i.e. pushing them to borrow *less* strongly). In particular, it changes the SPx prior stated in Section 2.2 in three ways:

1. for the historical borrowing submodel, the prior variance  $\sigma$  gets the less concentrated hyperprior

$$\sigma \sim TCauchy(0, 0.1, (0, \infty)),$$

whereas in the regular SPx method the scale parameter is 0.02,

2. for the regression submodel, the prior variance is not scaled down, so we just have

$$\theta_{reg} | \beta, \tau^2, \mathbf{x}_{H+1} \sim N(\beta^T \mathbf{x}_{H+1}, \tau^2),$$

whereas in the regular SPx the prior variance here is  $c\tau^2$  with  $c = \frac{1}{25}$ , and

3. the prior submodels weights are

$$(p_{hist}, p_{reg}, p_{ind}) = \left( \frac{1}{3}, \frac{1}{3}, \frac{1}{3} \right)$$

instead of  $(p_{hist}, p_{reg}, p_{ind}) = (\frac{1}{8}, \frac{1}{8}, \frac{3}{4})$  in the regular SPx.

In general, Table S1 suggests that the SPx model is robust to different reasonable choices of the prior. Results for the regular SPx (as presented in the text) and SPx C. and SPx D. are extremely similar in scenarios 2 and 3. In Scenarios 1 and 4, where either the external data are very helpful or very unhelpful, reveal some modest differences. Unsurprisingly, SPx C. performs slightly worse than the regular SPx in Scenario 1 since it is slightly less aggressive about borrowing from the external data. In contrast, SPx D. *does* beat out the regular SPx in Scenario 1, especially when the new trial is smaller ( $n_{max}^c = 100$ ), though it

does a bit worse in Scenario 4 (comparable to RMAP in Table 1). Here the prior in SPx D. is evidently not diffuse *enough* to compensate for the increased mass on the borrowing submodels, despite that its Cauchy scale parameter is 5 times larger than our basic prior. This suggests that the regular SPx strategy of making the borrowing submodels have tight priors while simultaneously putting most prior mass on the no-borrowing submodel is a good default choice.

### 3 Rationale for the SPx hyperprior

Near the end of Section 2.2 in the text, we highlighted two prior choices in SPx that drive its adaptive historical borrowing:

- (a) make the priors in the *hist* and *reg* submodels relatively strongly concentrated (i.e. high prior probability of small  $\sigma^2$  and  $\tau^2$ ), and
- (b) give relatively high prior weight to the *ind* (no-borrowing) submodel (i.e.  $p_{ind} > p_{hist}, p_{reg}$ ).

A more detailed explanation of these choices follows.

By posing quite informative priors for the *hist* and *reg* borrowing submodels, (a), we both allow strong borrowing when deemed appropriate (and  $p_{hist}^* + p_{reg}^*$  is large) and make the marginal likelihoods of these submodels more sensitive to conflict between the new and historical data. This means that their marginal likelihoods will more quickly dwarf the no-borrowing submodel’s marginal likelihood as borrowing grows safer and shrink compared to it when borrowing grows more dangerous. The rationale for *a priori* favoring the no-borrowing submodel, (b), is to compensate for the behavior of the three submodels’ marginal likelihoods in the challenging setting of moderate but not necessarily obvious conflict between the new and historical data. In this case, especially when the new trial size is small (e.g. at interim), the marginal likelihood of the no-borrowing submodel may not be much larger than that of the borrowing submodels because its prior is more diffuse and thus still gives nontrivial prior mass to response rates that have low likelihoods, so to get large  $p_{ind}^*$  in this case we must have large  $p_{ind}$ . This also reflects the idea that we should be conservative about historical

|                   | $n_{\max}^c = 150$ |        |        |        |        |        |       | $n_{\max}^c = 80$ |        |        |        |        |        |       |
|-------------------|--------------------|--------|--------|--------|--------|--------|-------|-------------------|--------|--------|--------|--------|--------|-------|
|                   | SPx                |        | SPx C. |        | SPx D. |        | Ind.  | SPx               |        | SPx C. |        | SPx D. |        | Ind.  |
|                   | Fixed              | Adapt. | Fixed  | Adapt. | Fixed  | Adapt. | Fixed | Fixed             | Adapt. | Fixed  | Adapt. | Fixed  | Adapt. | Fixed |
| <b>Scenario 1</b> |                    |        |        |        |        |        |       |                   |        |        |        |        |        |       |
| Size              | 200                | 160.3  | 200    | 164.7  | 200    | 153.5  | 200   | 100               | 80.5   | 100    | 82.4   | 100    | 76.6   | 100   |
| RMSE              | 0.018              | 0.018  | 0.020  | 0.020  | 0.016  | 0.016  | 0.029 | 0.022             | 0.022  | 0.026  | 0.025  | 0.017  | 0.017  | 0.037 |
| Coverage          | 98.8               | 98.9   | 98.1   | 98.2   | 99.0   | 99.0   | 93.5  | 99.3              | 99.2   | 98.8   | 99.1   | 99.8   | 99.7   | 96.3  |
| Width             | 0.086              | 0.094  | 0.092  | 0.101  | 0.082  | 0.090  | 0.110 | 0.117             | 0.130  | 0.128  | 0.141  | 0.104  | 0.114  | 0.154 |
| <b>Scenario 2</b> |                    |        |        |        |        |        |       |                   |        |        |        |        |        |       |
| Size              | 200                | 186.9  | 200    | 191.9  | 200    | 179.1  | 200   | 100               | 93.7   | 100    | 96.0   | 100    | 89.1   | 100   |
| RMSE              | 0.032              | 0.032  | 0.032  | 0.032  | 0.031  | 0.032  | 0.034 | 0.049             | 0.050  | 0.049  | 0.051  | 0.047  | 0.050  | 0.051 |
| Coverage          | 96.0               | 96.0   | 95.5   | 95.9   | 96.8   | 96.7   | 94.5  | 94.6              | 94.9   | 94.5   | 94.2   | 94.7   | 95.4   | 94.3  |
| Width             | 0.130              | 0.134  | 0.132  | 0.135  | 0.128  | 0.134  | 0.137 | 0.184             | 0.190  | 0.187  | 0.191  | 0.179  | 0.189  | 0.191 |
| <b>Scenario 3</b> |                    |        |        |        |        |        |       |                   |        |        |        |        |        |       |
| Size              | 200                | 168.0  | 200    | 172.6  | 200    | 162.9  | 200   | 100               | 82.3   | 100    | 84.4   | 100    | 78.6   | 100   |
| RMSE              | 0.025              | 0.026  | 0.026  | 0.026  | 0.025  | 0.025  | 0.029 | 0.032             | 0.033  | 0.034  | 0.034  | 0.031  | 0.033  | 0.040 |
| Coverage          | 93.3               | 94.9   | 93.7   | 95.0   | 94.3   | 94.7   | 94.2  | 95.7              | 95.3   | 95.6   | 95.5   | 96.0   | 95.8   | 95.3  |
| Width             | 0.097              | 0.103  | 0.101  | 0.108  | 0.098  | 0.106  | 0.110 | 0.129             | 0.140  | 0.137  | 0.148  | 0.128  | 0.141  | 0.155 |
| <b>Scenario 4</b> |                    |        |        |        |        |        |       |                   |        |        |        |        |        |       |
| Size              | 200                | 204.7  | 200    | 202.5  | 200    | 208.2  | 200   | 100               | 104.5  | 100    | 102.9  | 100    | 105.6  | 100   |
| RMSE              | 0.035              | 0.035  | 0.035  | 0.034  | 0.037  | 0.036  | 0.035 | 0.050             | 0.050  | 0.049  | 0.049  | 0.054  | 0.055  | 0.047 |
| Coverage          | 95.2               | 95.5   | 95.3   | 95.5   | 94.5   | 93.9   | 95.3  | 95.8              | 95.2   | 95.8   | 94.9   | 94.0   | 93.4   | 97.0  |
| Width             | 0.138              | 0.136  | 0.137  | 0.136  | 0.139  | 0.136  | 0.137 | 0.197             | 0.192  | 0.195  | 0.192  | 0.200  | 0.194  | 0.191 |

**Table S1:** Control group size and Frequentist estimation accuracy for the new trial’s control response rate, averaged over 1,000 simulated trials. Metrics are defined as in Table 1.

borrowing, especially when sample sizes are small.
